# Supplementary material for: Learning Correspondence for Deformable Objects
Source: arXiv:2405.08996 source file (2024-05-28)
Supplement: Supplementary file 2 [file appendix2_bakcup.tex]

%!TEX root = ../main.tex

\begin{theorem}[Expectation-Maximization Guarantee]
\label{thm:EMrepeat}
In the setting of Definition \ref{set:problem}, 
assume that the initial clustering $\cH$ is 
$(\tau,\alpha,m_0)$-good in the sense of Definition \ref{def:initial_conditions}, where $m_0 \geq 2.5 \cdot 10^8  (\frac{\alpha+1}{\alpha-1})^2 \log \frac {18} {\delta} \max\left\{\frac{B^4}{\lambda^2},  B^2 , \sigma, 0.1  \right\}$ 
% is some sufficiently large polynomial function of $1/\alpha, 1/\sigma_j$ and $\log(1/\delta)$, 
where $\delta$ is the probability of failure of the algorithm and $\lambda$ is the smallest eigenvalue of {$\frac 1 m \sum_i \va'_i (\va'_i)\tran$.}
Then, the partition $\cH'$ returned by \Cref{alg:EM} {recovers each of the ground truth clusters} (\eg the objects and background) with probability $1-\delta$.
% Then, running \Cref{alg:EM}, with probability $1-\delta$,
% returns $\cH'$, a partition of the set of correspondences $S$, {recovering each of the ground truth clusters} (\ie the objects and background). 
\end{theorem}
% We now sketch a proof outline of our main theoretical guarantee. 
% \emph{Intuition:}
% The proof of~\cref{thm:EM} follows by noting that the initial clustering results in a partition of each ground truth cluster such that one of the partitions is notably larger than the rest. 
% As the algorithm progresses, the M-step assigns more points to the biggest estimated cluster until it is exactly matches to the ground truth object which contains it. 
% This happens because the likelihood term $W_{i,j;\tau}$ is dominated by the weight term $\pi_j$ of the largest cluster. 

\emph{Proof:}
We make the following observations, which together imply that the final clusters produced by~\Cref{thm:EM}  recover the ground truth clusters. 
First, {each ground truth-cluster is partitioned by the initial clustering}. This is because
% one element of which is $\alpha$-times larger than all the others.
the $\tau$-connected subsets of the data either consist of samples that are entirely contained in one of the $G_j$ or (possibly) the set of outliers. Since the initial clustering $\cH$ exclusively consists of $\tau$-connected subsets, % and is a partition of $S$, 
each element of $\cH$ is either a subset of $G_j$ for some $j$ or entirely consists of outliers.

Now %now set up some convention for what follows.
suppose the weights for the clusters are given by $\pi_1, \dots, \pi_{K}$.
Without loss of generality, suppose $\{ H_1, \dots, H_t \}$ form a partition of $G_1$ 
with $\pi_1 \geq \dots \geq \pi_{t}$. Since $\cH$ is $(\tau,\alpha, m_0)$-good,
we know that $\pi_1 > \alpha \pi_2$ because of \Cref{item:identifying-cluster} in Definition~\ref{def:initial_conditions}. 
Our second claim is that in each iteration of the $M$-step,
elements of $S$ that are $\tau$-close to the largest cluster $H_1$ are assigned to $H_1$. 
To see this, consider a point $(\va_i, \vb_i) \in G_1 \setminus H_1$ which is $\tau$-close to $H_{1}$ (if no such point exists, then $H_1 = G_1$). We show that for the point $(\va_i, \vb_i)$, the likelihood term $W_{i,j;\tau}$ is maximized when $j=1$. 
% This will follow from the fact that $W_{i,1;\tau}$ is much larger than $W_{i,j;\tau}$ for all $j\in[t] \setminus \{1\}$ because $\pi_1$ is much larger than the weights for the other clusters.

% Since Horn's Method is consistent (to be consistent means that with a sufficiently large sample size, the algorithm converges to the true solution in the presence of zero-mean  noise) and the domain of the point-cloud is bounded by a ball of radius $B$, 
% $(\hat{\MR}_j^{(r)}, \hat{\vt}_j^{(r)})$ and $\sigma_j$ estimates $(\MR_j^{(r)}, \vt_j^{(r)})$ and $\sigma_j$ up to an additive error of $100c'$. Let $m_0 := \frac
% {2 \log \frac 2 \delta}
% {(-\frac{4B}{\sigma_j} -\frac{2 B^2}{\sigma_j \lambda} +  \sqrt{(\frac{4B}{\sigma_j} + \frac{2 B^2}{\sigma_j \lambda} )^2 - \frac{1}{2400} \frac{1-\alpha}{1+\alpha} \frac{1}{\sigma_j} })^2}$.

% \red{A large sample size can be ensured by letting $m_0$ be a sufficiently large polynomial function of $1/\eta', 1/\sigma_j$, and $\log(1/\delta)$, where $\delta$ is the probability of success.} 
% Then, for all $H_j$ such that $|H_j|$ is large enough, our estimates $h_j$ and $\sigma_j$ converge to the corresponding ground truth parameters ($g_1$ and $\sigma_j$).

% However, if $|H_j|$ is much smaller than $m_\min$ \new{as defined in our algorithm}, we delete the cluster $H_j$ from our set of candidate clusters. 

We use Horn's method to obtain the estimated $\hat \MR_j$ and $\hat \vt_j$. Let $\vv_{i, j} := \hat{\MR}_j \va_i + \hat{\vt}_j - (\MR_j \va_i + \vt_j)$ which is the estimation error given by the estimated pose $(\hat \MR, \hat \vt)$ as compared to the ground truth pose $(\MR, \vt)$, then we can get the estimated noise variance $\hat\sigma_j$, \ie \red{$\frac 1 3 \sum_{k=1}^3 \left (\frac 1 n \sum_{i=1}^n (\epsilon_{i,j,k} - \frac 1 n \sum_{i=1}^n \epsilon_{i,j,k})^2 \right)$}. Notice that 
$\argmax_j W_{i,j;\tau} 
= \argmax_j \pi_j \phi_j(\vb_i \mid \va_i) 
= \argmax_j \pi_j / (\hat\sigma_j)^3 \exp(-\norm{\vb_i - \hat{\MR}_j\va_i - \hat{\vt}_j }^2/(2 {\hat\sigma_j}^2)) $ (where we dropped constants that are inconsequential for the maximization). 
\LC{missing $\frac{1}{2}$ (does it matter?) and $\hat\sigma_j$ should be $\hat\sigma_j^3$}

Let $C = \sigma_j / \hat\sigma_j$. Then, we have
% \begin{align}
%     \hat\sigma = \sigma + \hat\sigma - \sigma = \sigma * (1 + (\hat\sigma - \sigma) / \sigma)
% \end{align}

\begin{align}
&\quad \frac{\pi_j}{(\hat\sigma_j)^3} \exp\left(-\frac{\norm{\vb_i - \hat{\MR}_j \va_i - \hat{\vt}_j }^2}{ 2\hat\sigma_j^2}\right) \\
&= \frac{C^3 \pi_j}{\sigma_j^3} \exp\left(-C^2\frac{\norm{\vb_i - \MR_j \va_i - \vt_j + \vv_{i, j}}^2}{ 2\sigma_j^2}\right) \\
&= \frac{C^3 \pi_j}{\sigma_j^3} \exp\left(-C^2\frac{2 \vv_{i, j} \cdot (\vb_i - \MR_j \va_i - \vt_j) + \norm{\vv_{i, j}}^2}{ 2\sigma_j^2}\right) \\
&\quad \cdot \exp\left(- C^2 \frac{\norm{\vb_i - \MR_j \va_i - \vt_j}^2}{ 2\sigma_j^2}\right) \\
&= \frac{C^3 \pi_j}{\sigma_j^3} \exp\left(-C^2\frac{2 \vv_{i, j} \cdot (\vb_i - \MR_j \va_i - \vt_j) + \norm{\vv_{i, j}}^2}{ 2\sigma_j^2}\right) \\
&\quad \cdot \exp\left(- (C^2 - 1) \frac{\norm{\vb_i - \MR_j \va_i - \vt_j}^2}{ 2\sigma_j^2}\right) \\
&\quad \cdot \exp\left(- \frac{\norm{\vb_i - \MR_j \va_i - \vt_j}^2}{ 2\sigma_j^2}\right)
\end{align}
% Let $c = \frac{|\hat \sigma_j - \sigma_j|}{\sigma_j}$ such that 
We have $C = \frac{\sigma_j}{\hat \sigma_j + \sigma_j - \sigma_j} = \frac{1}{1 + \frac{\hat \sigma_j - \sigma_j}{\sigma_j}} = \frac{1}{1 \pm \frac{|\hat \sigma_j - \sigma_j|}{\sigma_j}} $
% = \frac{1}{1 \pm c}$.
Then, we have, for $\frac{|\hat \sigma_j - \sigma_j|}{\sigma_j} \in (0, 0.5)$, $1 - 2\frac{|\hat \sigma_j - \sigma_j|}{\sigma_j} \leq C \leq 1 + 2\frac{|\hat \sigma_j - \sigma_j|}{\sigma_j}$.
Since $\max_i ||\vv_{i,j}|| \geq |\hat \sigma_j - \sigma_j|$, then $1 - 2\frac{\max_i ||\vv_{i,j}||}{\sigma_j} \leq C \leq 1 + 2\frac{\max_i ||\vv_{i,j}||}{\sigma_j}$. Let $c = \frac{\max_i ||\vv_{i,j}||}{\sigma_j}$ such that $1 - 2c \leq C \leq 1 + 2c$.
Lemma~\ref{lem:close_to_1} shows that except for $(\pi_j/\sigma_j^3)~\exp(-\frac{\norm{\vb_i - \MR_j \va_i - \vt_j}^2}{2\sigma_j^2})$, all the other terms take values in $[1 - 100 c, 1 + 100 c]$. 
\begin{lemma}\label{lem:sigma_ratio}
In the setting of \Cref{thm:EM}, if $m \geq 2 \cdot 10^3 \log{\frac 2 \delta}$, then with probability $1-\delta$, $\frac 1 {\sqrt{3}} - 2 \sqrt[4]{\frac 2 {3m} \log{\frac 2 \delta}} &\leq \frac{\sigma_j}{\sigma} &\leq \frac 1 {\sqrt{3}} + 2 \sqrt[4]{\frac 2 {3m} \log{\frac 2 \delta}}$. 
\end{lemma}
\begin{proof}
\begin{align}
&~|\sigma_j^2 - \E[\sigma_j^2]| \\
&\quad \color{gray} \text{(using variance of uniform distribution $[-\sigma, \sigma]$)} \\
&= |\sigma_j^2 - \frac 1 3 \sigma^2| \\
&\quad \color{gray} \text{(using definition of $\sigma_j$)} \\
&= \left |\frac 1 3 \sum_{k=1}^3 \left (\frac 1 m \sum_{i=1}^m (\epsilon_{i,j,k} - \frac 1 m \sum_{i=1}^m \epsilon_{i,j,k})^2 \right) - \frac 1 3 \sigma^2 \right | \\
&\quad \color{gray} \text{(applying Hoeffding's inequality \ref{thm:hoeffding})} \\
&\leq 4 \sigma^2 \sqrt{\frac 2 {3m} \log{\frac 2 \delta}}
\end{align}
We can use this to find the upper and lower bound for $\frac{\sigma_j}{\sigma}$. Since $m \geq 2 \cdot 10^3 \log{\frac 2 \delta}$, we have $\frac 1 {\sqrt{3}} > 2 \sqrt[4]{\frac 2 {3m} \log{\frac 2 \delta}}$. Then, we have
\begin{align}
\frac 1 3 \sigma^2 - 4 \sigma^2 \sqrt{\frac 2 {3m} \log{\frac 2 \delta}} &\leq \sigma_j^2 &\leq \frac 1 3 \sigma^2 + 4 \sigma^2 \sqrt{\frac 2 {3m} \log{\frac 2 \delta}} \\
\frac 1 3 - 4 \sqrt{\frac 2 {3m} \log{\frac 2 \delta}} &\leq \frac{\sigma_j^2}{\sigma^2} &\leq \frac 1 3 + 4 \sqrt{\frac 2 {3m} \log{\frac 2 \delta}} \\
\frac 1 {\sqrt{3}} - 2 \sqrt[4]{\frac 2 {3m} \log{\frac 2 \delta}} &\leq \frac{\sigma_j}{\sigma} &\leq \frac 1 {\sqrt{3}} + 2 \sqrt[4]{\frac 2 {3m} \log{\frac 2 \delta}}
\end{align}
\end{proof}
By letting $m \geq 2\cdot 10^7 \log{\frac 2 \delta} > 2 \cdot 10^3 \log{\frac 2 \delta}$, using \Cref{lem:sigma_ratio}, with probability $1-\delta$, we have $\frac 1 2 \leq \frac{\sigma_j}{\sigma} \leq 1$, i.e. $1 \leq \frac{\sigma}{\sigma_j} \leq 2$.
\begin{lemma}\label{lem:close_to_1}
In the setting of \Cref{thm:EM}, if $C = 1 \pm (c/2)$, $c \in (0, 0.03)$ and $m \geq 2\cdot 10^7 \log{\frac 2 \delta}$, then with probability $1-\delta$, $C^3 \cdot \exp(-C^2~\frac{( 2 \vv_{i, j}) \cdot (\vb_i - \MR_j \va_i - \vt_j) + \norm{\vv_{i, j}}^2}{2 \sigma_j^2}) \cdot \exp(-(C^2 - 1)~\frac{\norm{\vb_i - \MR_j \va_i - \vt_j}^2}{2\sigma_j^2}) \in [1 - 100 c, 1 + 100 c]$. 
\end{lemma}
\begin{proof}
We already know that $1- 2c \leq C \leq 1 + 2c$. We will show the following:\\
(1) $|1 - \exp(-C^2~\frac{(2 \vv_{i, j}) \cdot (\vb_i - \MR_j \va_i - \vt_j) + \norm{\vv_{i, j}}^2}{\sigma_j^2})| \leq (1+2c)^2 \left (8c + c^2\right)$, \\
(2) $|1 - \exp(-(C^2-1)~\frac{\norm{\vb_i - \MR_j \va_i - \vt_j}^2}{\sigma_j^2})| \leq 48(c + c^2)$. \\
To this end, we will need the following fact: for all $|p| \leq 1$,   $1 - 2|p|\leq \exp(p) \leq 1+ 2 |p|$. \\
Note that since the noise is bounded in absolute value by $\sigma$, we have $\norm{\vb_i - \MR_j \va_i - \vt_j} < \sqrt{3} \sigma$. By \Cref{lem:sigma_ratio}, we have $1 \leq \frac{\sigma}{\sigma_j} \leq 2$.
% We will show that $\exp(-C^2~\frac{(\pm 2 \eta') \cdot (\vb_i - R_j \va_i - \vt_j) + \norm{\eta'}^2}{\sigma_j^2}) = 1 +\eta_1$ and $\exp(-(2(C-1) + (C-1)^2)~\frac{\norm{\vb_i - R_j \va_i - \vt_j}^2}{\sigma_j^2}) = 1+\eta_2$ such that $\eta_1, \eta_2$ are both $O(c)$ where 
Together, these imply, 
\begin{align}
&\left|1-\exp\left(-C^2~\frac{(2 \vv_{i, j}) \cdot (\vb_i - \MR_j \va_i - \vt_j) + \norm{\vv_{i, j}}^2}{2\sigma_j^2}\right)\right|\\
&\leq 2\left |-C^2~\frac{(2 \vv_{i, j}) \cdot (\vb_i - \MR_j \va_i - \vt_j) + \norm{\vv_{i, j}}^2}{2\sigma_j^2} \right| \\
& \leq 2C^2 \left ( \left |\frac{2 \vv_{i, j} \cdot (\vb_i - \MR_j \va_i - \vt_j)}{2\sigma_j^2}\right| + \frac{\norm{\vv_{i, j}}^2}{2\sigma_j^2}\right) \\
& \leq 2C^2 \left (\frac{2 \norm{\vv_{i, j}} \norm{\vb_i - \MR_j \va_i - \vt_j}}{2\sigma_j^2} + \frac{\norm{\vv_{i, j}}^2}{2\sigma_j^2}\right) \\
& \leq C^2 \left (\frac{2 \norm{\vv_{i, j}} \sqrt{3} \sigma}{\sigma_j^2} + \frac{\norm{\vv_{i, j}}^2}{\sigma_j^2}\right) \\
& \leq (1+2c)^2 \left (2 \sqrt{3} c \frac{\sigma}{\sigma_j} + c^2\right) \\
& \leq (1+2c)^2 \left (8c + c^2\right) \\
% & \leq 10c
% & \leq 2C^2 \left (\frac{2 \eta'_j \norm{\vb_i - \MR_j \va_i - \vt_j}}{2\sigma_j^2} + \frac{(\eta'_j)^2}{2\sigma_j^2}\right) \\
% & \leq 2C^2 \left (\frac{2 \norm{\eta'} \sqrt{3} \sigma_j}{\sigma_j^2} + \frac{\norm{\eta'}^2}{\sigma_j^2} \right) \\
% & \leq 2C^2 \left (\frac{2 \sqrt{3} \norm{\eta'}}{\sigma_j} + \frac{\norm{\eta'}^2}{\sigma_j^2} \right)\\
% & \leq \frac{1}{(1-c)^2}\left(\sqrt{3} c + \frac 1 2 c^2 \right)
% \frac{2 \sqrt{3} \norm{\eta'}}{\sigma_j} + \frac{\norm{\eta'}^2}{\sigma_j^2} \right)
\end{align}
Similarly, we can show that
\begin{align}
&\left | 1-\exp\left(-(C^2-1)~\frac{\norm{\vb_i - \MR_j \va_i - \vt_j}^2}{2\sigma_j^2}\right) \right|\\
% &\leq 2\left|-(2(C-1) + (C-1)^2)~\frac{\norm{\vb_i - R_j \va_i - \vt_j}^2}{\sigma_j^2}\right| \\
&\leq |2(C^2- 1)~\frac{3 \sigma^2}{2 \sigma_j^2}| \\
&\leq 3|((1+2c)^2- 1)~\frac{ \sigma^2}{ \sigma_j^2}| \\
&\leq 3|(1 + 4c + 4c^2- 1)~\frac{ \sigma^2}{ \sigma_j^2}| \\
&\leq 3(4c + 4c^2)~\frac{ \sigma^2}{ \sigma_j^2} \\
&\leq 12(c + c^2)~\frac{ \sigma^2}{ \sigma_j^2} \\
&\leq 48(c + c^2) \\
\end{align}
Putting everything together,
% $\frac{c}{c \pm 1} = 1 - \frac{\eta'/\sigma_j}{\eta'/\sigma_j \pm 1} = 1 - \frac{\eta'}{\eta' \pm \sigma_j} = 1 + \eta_0$. 
we have $C^3 \cdot \exp(-C^2~\frac{( 2 \vv_{i, j}) \cdot (\vb_i - \MR_j \va_i - \vt_j) + \norm{\vv_{i, j}}^2}{\sigma_j^2}) \cdot \exp(-(C^2 -1)~\frac{\norm{\vb_i - \MR_j \va_i - \vt_j}^2}{\sigma_j^2}) \in [(1 - 2c)^3 (1 - (1+2c)^2 (8c+c^2)) (1 - 48(c+c^2)), (1 + 2c)^3 (1 + (1+2c)^2 (8c+c^2)) (1 + 48(c+c^2))] \in [1 - 100c, 1 + 100 c]$ for $c\in(0, 0.03)$.
\end{proof}
We choose $c$ to be sufficiently small so that $100c  \leq \frac{\alpha-1}{\alpha+1} $.
% To enforce this, i.e. that the final error is smaller than $\eta'_j \leq \frac{\sigma_j}{33} \frac{\alpha -1}{\alpha+1}$ we will bound each of the contributions to the final error according to  
Recall that \Cref{lem:HornRepeat} states that 
\begin{align*}
\|\hat \MR - \MR\|_F^2 \leq \frac {18 B \sigma}{\lambda_{min}(\MSigma)}\sqrt{\frac{2}{m} \log \frac {\textcolor{red}{18}} \delta }
\end{align*}
and,
\begin{align*}
\| \hat \vt - \vt \|_2^2 \leq  36 B \sigma  \sqrt{\frac{2}{m} \log \frac {\textcolor{red}{18}} \delta } +
\frac{12}{m} \sigma^2 \log \frac {\textcolor{red}{6}} \delta 
\end{align*}
Since the largest final error of $\vv_{i,j} = \norm{\vb_i - \MR_j \va_i - \vt_j}^2$ for all $i$ is bounded by the largest possible error given by \Cref{lem:HornRepeat}, then $\max_i \|\vv_{i,j}\|$ may be bounded by $\frac {18 B^2 \sigma}{\lambda_{min}(\MSigma)}\sqrt{\frac{2}{m} \log \frac {\textcolor{red}{18}} \delta } + 36 B \sigma  \sqrt{\frac{2}{m} \log \frac {\textcolor{red}{18}} \delta } +
\frac{12}{m} \sigma^2 \log \frac {\textcolor{red}{6}} \delta$. Then, since $\frac{\sigma}{\sigma_j} \leq 2$, we have $\frac{\sigma}{2}c  = \frac{\sigma}{2} \frac{\max_i \|\vv_{i,j}\|}{\sigma_j} \leq \max_i \|\vv_{i,j}\|$ which tells us $c \leq \frac {36 B^2 }{\lambda_{min}(\MSigma)}\sqrt{\frac{2}{m} \log \frac {\textcolor{red}{18}} \delta } + 72 B  \sqrt{\frac{2}{m} \log \frac {\textcolor{red}{18}} \delta } + \frac{24}{m} \sigma \log \frac {\textcolor{red}{6}} \delta$. We will solve for $m$ satisfying (1) $\frac {18 B^2}{\lambda_{min}(\MSigma)}\sqrt{\frac{2}{m} \log \frac {\textcolor{red}{18}} \delta }  < \frac 1 3 \frac{1}{100} \frac{\alpha-1}{\alpha+1}$, (2) $36 B  \sqrt{\frac{2}{m} \log \frac {\textcolor{red}{18}} \delta } < \frac 1 3 \frac{1}{100} \frac{\alpha-1}{\alpha+1}$ and (3) $\frac{12}{m} \sigma \log \frac {\textcolor{red}{6}} \delta < \frac 1 3 \frac{1}{100} \frac{\alpha-1}{\alpha+1}$. Any $m$ simultaneously satisfying (1), (2), (3), and \Cref{lem:sigma_ratio} will give us our result. To this end, we just choose $m_0$ to be the largest of these $m$.
which is enforced by 
$m_0 \geq 2.5 \cdot 10^8  (\frac{\alpha+1}{\alpha-1})^2 \log \frac{18}{\delta} \max 
\{ \frac{B^4}{\lambda^2},  B^2 , \sigma , 0.1\} > 
2.5 \cdot 10^8 \max \{\frac{B^4}{\lambda^2} (\frac{\alpha+1}{\alpha-1})^2 \log \frac {18} {\delta},  B^2 
(\frac{\alpha+1}{\alpha-1})^2 \log \frac{18}{\delta}, \sigma \frac{\alpha+1}{\alpha-1}
\log \frac{6}{\delta}, \\ 0.1 \log \frac{2}{\delta} \}$, 
using Theorem \ref{lem:HornRepeat}, we get, $100c \leq \frac{\alpha -1}{\alpha+1}$.
% (\frac
% {24 \sigma_j \log \frac {18} {\delta}}
% {- ( \frac{18 B^2}{\lambda} + 36B) \sqrt{2 \log \frac{2}{\delta}} + \sqrt{( \frac{18 B^2}{\lambda} + 36B)^2 {2 \log \frac{2}{\delta}} + \frac {3} {25} \sigma_j (\log \frac{18}{\delta}) \frac{\alpha-1}{\alpha+1}}} )^2

% \new{Constraints: 
% 1. $\eta' = c \sigma_j$ then $C = 1/(1 \pm c)$.
% 2. $c$ can be chosen to be a sufficiently small constant (like $0.1$) since $\sigma_j =1$. This will reduce $\eta'$.
% The cost of this is the sample size. 

% }

 % we see that for a sufficiently large $H_j$ for $j \in [t]$, 
 % $h_j$ converges to $g_1$ on the domain of the point-cloud, 
 % i.e. $|h_j(\va_i) - g_1(\va_i)| \leq \eta'$. 

% Similarly, it can be shown that our estimate of the standard deviation of the noise is also correct upto an additive error of $\eta'$.
% true for our estimate of the standard deviation of the noise.

% Let $\sigma_j$ denote the standard deviation of the noise in $G_1$ with respect to the ground truth rotation and translation $g_1$. 
 
% (the bound on the norm of the elements of the point cloud). 

\new{SK: Still hand-wavy.}
Since $\exp(-\norm{\vb_i - g_1(\va_i)}^2/{\sigma_j}^2)/\sigma_j^3$ is roughly a constant with respect to $j$ (by \Cref{lem:sigma_ratio}) in $\argmax_j W_{i,j;\tau}= \argmax_j \pi_j (1\pm 100c) \exp(-\norm{\vb_i - g_1(\va_i)}^2/{\sigma_j}^2)/\sigma_j$, it does not affect the maximization. 
This implies 
% $\argmax_j W_{i,j;\tau}=\argmax_j \pi_j (1\pm 3\eta)$, and so 
$\argmax_j W_{i,j;\tau}$ is essentially determined by $\argmax_j \pi_j (1\pm 100c)$. By letting large enough $m_0$ ,we have small $100c$ to ensure $(1+100c)/(1-100c) < \alpha$ and recalling that $\pi_1 > \alpha \pi_2$, we see $\argmax_j W_{i,j;\tau} = \argmax_j \pi_j (1\pm 100c) = 1$. Since $\pi_1$ keeps increasing in size in each iteration, eventually all the elements of $G_1$ will collect into $H_1$. 

% $\exp(-\norm{g_1(\va_i) - \vb_i}^2/{{\sigma_j^*}_1}^2)/{\sigma_j^*}_1$ for $\eta$ chosen to be sufficiently small. Since the second term is a constant with respect to $j$, by choosing $\eta$ to be sufficiently small we can ensure $(1+\eta)/(1-\eta) < \alpha$, and so $\argmax_j W_{i,j;\tau} = \argmax_j \pi_j (1\pm \eta) = 1$. 
% (i.e. smaller than $(1-\alpha)(1/3)$)
% $\argmax_j W_{i,j;\tau} 
% = \argmax_j \pi_j \phi_j(\vb_i \mid \va_i) 
% = \argmax_j \pi_j \exp(-\norm{h_j(\va_i) - \vb_i}^2/{\sigma_j}^2)/\sigma_j 
% = \argmax_j \pi_j (1\pm \eta') \exp(-\norm{g_1(\va_i) - \vb_i}^2/{{\sigma_j^*}_1}^2)/{\sigma_j^*}_1 
% = 1$. 
% The second-to-last equality is a consequence of choosing $\eta$ sufficiently small,
% and $\eta'$ satisfying $1+\eta' < \alpha$. 
\qed
