# Supplementary material for: Learning Correspondence for Deformable Objects
Source: arXiv:2405.08996 source file (2024-05-28)
Supplement: Supplementary file 3 [file appendix2.tex]

%!TEX root = ../main.tex

\begin{theorem}[Expectation-Maximization Guarantee]
\label{thm:EM}
In the setting of Definition \ref{set:problem}, 
assume that the initial clustering $\cH$ is 
$(\tau,\alpha,m_0)$-good in the sense of Definition \ref{def:initial_conditions}, where $m_0 \geq 2.5 \cdot 10^4 \log \frac{18}{\delta} \max 
\{ \frac{B^4}{\lambda^2},  B^2 , \sigma\} (\frac 1 2 \log \frac{\alpha}{8})^{-\frac 1 2}$ 
% is some sufficiently large polynomial function of $1/\alpha, 1/\sigma_j$ and $\log(1/\delta)$, 
where $\delta$ is the probability of failure of the algorithm and $\lambda$ is the smallest eigenvalue of {$\frac 1 m \sum_i \va'_i (\va'_i)\tran$.}
Then, the partition $\cH'$ returned by \Cref{alg:EM} {recovers each of the ground truth clusters} (\eg the objects and background) with probability $1-\delta$.
% Then, running \Cref{alg:EM}, with probability $1-\delta$,
% returns $\cH'$, a partition of the set of correspondences $S$, {recovering each of the ground truth clusters} (\ie the objects and background). 
\end{theorem}
% We now sketch a proof outline of our main theoretical guarantee. 
% \emph{Intuition:}
% The proof of~\cref{thm:EM} follows by noting that the initial clustering results in a partition of each ground truth cluster such that one of the partitions is notably larger than the rest. 
% As the algorithm progresses, the M-step assigns more points to the biggest estimated cluster until it is exactly matches to the ground truth object which contains it. 
% This happens because the likelihood term $W_{i,j;\tau}$ is dominated by the weight term $\pi_j$ of the largest cluster. 

\emph{Proof:}
We make the following observations, which together imply that the final clusters produced by~\Cref{alg:EM}  recover the ground truth clusters. 
First, {each ground truth-cluster is partitioned by the initial clustering}. This is because
% one element of which is $\alpha$-times larger than all the others.
the $\tau$-connected subsets of the data either consist of samples that are entirely contained in one of the $G_j$ or (possibly) the set of outliers. Since the initial clustering $\cH$ exclusively consists of $\tau$-connected subsets, % and is a partition of $S$, 
each element of $\cH$ is either a subset of $G_j$ for some $j$ or entirely consists of outliers.

Now %now set up some convention for what follows.
suppose the weights for the clusters are given by $\pi_1, \dots, \pi_{K}$.
Without loss of generality, suppose $\{ H_1, \dots, H_t \}$ form a partition of $G_1$ 
with $\pi_1 \geq \dots \geq \pi_{t}$. Since $\cH$ is $(\tau,\alpha, m_0)$-good,
we know that $\pi_1 > \alpha \pi_2$ because of \Cref{item:identifying-cluster} in Definition~\ref{def:initial_conditions}. 
Our second claim is that in each iteration of the $M$-step,
elements of $S$ that are $\tau$-close to the largest cluster $H_1$ are assigned to $H_1$. 
To see this, consider a point $(\va_i, \vb_i) \in G_1 \setminus H_1$ which is $\tau$-close to $H_{1}$ (if no such point exists, then $H_1 = G_1$). We show that for the point $(\va_i, \vb_i)$, the likelihood term $W_{i,j;\tau}$ is maximized when $j=1$. 
% This will follow from the fact that $W_{i,1;\tau}$ is much larger than $W_{i,j;\tau}$ for all $j\in[t] \setminus \{1\}$ because $\pi_1$ is much larger than the weights for the other clusters.

% Since Horn's Method is consistent (to be consistent means that with a sufficiently large sample size, the algorithm converges to the true solution in the presence of zero-mean  noise) and the domain of the point-cloud is bounded by a ball of radius $B$, 
% $(\hat{\MR}_j^{(r)}, \hat{\vt}_j^{(r)})$ and $\sigma_j$ estimates $(\MR_j^{(r)}, \vt_j^{(r)})$ and $\sigma_j$ up to an additive error of $100c'$. Let $m_0 := \frac
% {2 \log \frac 2 \delta}
% {(-\frac{4B}{\sigma_j} -\frac{2 B^2}{\sigma_j \lambda} +  \sqrt{(\frac{4B}{\sigma_j} + \frac{2 B^2}{\sigma_j \lambda} )^2 - \frac{1}{2400} \frac{1-\alpha}{1+\alpha} \frac{1}{\sigma_j} })^2}$.

% \red{A large sample size can be ensured by letting $m_0$ be a sufficiently large polynomial function of $1/\eta', 1/\sigma_j$, and $\log(1/\delta)$, where $\delta$ is the probability of success.} 
% Then, for all $H_j$ such that $|H_j|$ is large enough, our estimates $h_j$ and $\sigma_j$ converge to the corresponding ground truth parameters ($g_1$ and $\sigma_j$).

% However, if $|H_j|$ is much smaller than $m_\min$ \new{as defined in our algorithm}, we delete the cluster $H_j$ from our set of candidate clusters. 

Let $(\MR, \vt)$ be the ground truth pose for $G_1$. We use Horn's method to obtain the estimated $\hat \MR_j$ and $\hat \vt_j$. Let $\vv_{i, j} := \hat{\MR}_j \va_i + \hat{\vt}_j - (\MR \va_i + \vt)$ which is the estimation error given by the estimated pose $(\hat \MR_j, \hat \vt_j)$ of $H_j$ as compared to the ground truth pose $(\MR, \vt)$ of $G_1$. Let the estimated noise variance $\hat\sigma_j = {\frac 1 3 \sum_{k=1}^3 \left (\frac 1 n \sum_{i=1}^n (\epsilon_{i,j,k} - \frac 1 n \sum_{i=1}^n \epsilon_{i,j,k})^2 \right)}$. Notice that 
$\argmax_j W_{i,j;\tau} 
= \argmax_j \pi_j \phi_j(\vb_i \mid \va_i) 
= \argmax_j \pi_j / (\hat\sigma_j)^3 \exp(-\norm{\vb_i - \hat{\MR}_j\va_i - \hat{\vt}_j }^2/(2 {\hat\sigma_j}^2)) $ (where we dropped constants that are inconsequential for the maximization). 
% \LC{missing $\frac{1}{2}$ (does it matter?) and $\hat\sigma_j$ should be $\hat\sigma_j^3$}

Let $C = \sigma / \hat\sigma_j$. Then, we have
% \begin{align}
%     \hat\sigma = \sigma + \hat\sigma - \sigma = \sigma * (1 + (\hat\sigma - \sigma) / \sigma)
% \end{align}

\begin{align}
&\quad \frac{\pi_j}{(\hat\sigma_j)^3} \exp\left(-\frac{\norm{\vb_i - \hat{\MR}_j \va_i - \hat{\vt}_j }^2}{ 2\hat\sigma_j^2}\right) \\
&= \frac{C^3 \pi_j}{\sigma^3} \exp\left(-C^2\frac{\norm{\vb_i - \MR \va_i - \vt + \vv_{i, j}}^2}{ 2\sigma^2}\right) \\
% &= \frac{C^3 \pi_j}{\sigma^3} \exp\left(-C^2\frac{2 \vv_{i, j} \cdot (\vb_i - \MR \va_i - \vt) + \norm{\vv_{i, j}}^2}{ 2\sigma^2}\right) \\
% &\quad \cdot \exp\left(- C^2 \frac{\norm{\vb_i - \MR \va_i - \vt}^2}{ 2\sigma^2}\right) \\
% &= \frac{C^3 \pi_j}{\sigma^3} \exp\left(-C^2\frac{2 \vv_{i, j} \cdot (\vb_i - \MR \va_i - \vt) + \norm{\vv_{i, j}}^2}{ 2\sigma^2}\right) \\
% &\quad \cdot \exp\left(- (C^2 - 1) \frac{\norm{\vb_i - \MR \va_i - \vt}^2}{ 2\sigma^2}\right) \\
% &\quad \cdot \exp\left(- \frac{\norm{\vb_i - \MR \va_i - \vt}^2}{ 2\sigma^2}\right)
\end{align}
% Let $c = \frac{|\hat \sigma_j - \sigma_j|}{\sigma_j}$ such that 
% We have $C = \frac{\sigma}{\hat \sigma_j + \sigma - \sigma} = \frac{1}{1 + \frac{\hat \sigma_j - \sigma}{\sigma}} = \frac{1}{1 \pm \frac{|\hat \sigma_j - \sigma|}{\sigma}} $
% % = \frac{1}{1 \pm c}$.
% Then, we have, for $\frac{|\hat \sigma_j - \sigma|}{\sigma} \in (0, 0.5)$, $1 - 2\frac{|\hat \sigma_j - \sigma|}{\sigma} \leq C \leq 1 + 2\frac{|\hat \sigma_j - \sigma|}{\sigma}$.
% Since $\max_i ||\vv_{i,j}|| \geq |\hat \sigma_j - \sigma_j|$, then $1 - 2\frac{\max_i ||\vv_{i,j}||}{\sigma_j} \leq C \leq 1 + 2\frac{\max_i ||\vv_{i,j}||}{\sigma_j}$. 
Let $c = \frac{\max_i ||\vv_{i,j}||}{\sigma}$. Then, the largest possible value without the weight $\pi_j$ is
$
\frac{C_{\max}^3}{\sigma^3}
$.
Note that $C$ approaches $\sqrt{3}$ as number of samples going to infinity. We can easily control $C$ to be between 1 and 2 with very high probability using Hoeffding's inequality. Thus, let $C_min = 1$ and $C_max = 2$ be the min and max of $C$ respectively.

Thus, to have the likelihood of cluster with $j=1$ always larger than the rest, we need to make sure
\begin{align}
\frac{\pi_1}{\pi_j} &\geq \frac{\frac{C_{\max}^3}{\sigma^3}}{\frac{C_{\min}^3}{\sigma^3}\exp(-C_{\max}^2\frac{\norm{\vb_i - \MR \va_i - \vt + \vv_{i, j}}^2}{ 2\sigma^2})} \\
&= \frac{C_{\max}^3}{C_{\min}^3} \exp(C_{\max}^2\frac{\norm{\vb_i - \MR \va_i - \vt + \vv_{i, j}}^2}{ 2\sigma^2}) \\
&= \frac{2^3}{1^3} \exp(2^2\frac{\norm{\vb_i - \MR \va_i - \vt + \vv_{i, j}}^2}{ 2\sigma^2}) \\
&= 8 \exp(2\frac{\norm{\vb_i - \MR \va_i - \vt + \vv_{i, j}}^2}{\sigma^2}),
\end{align}
Since 
\begin{align}
&\quad \exp(2\frac{\norm{\vb_i - \MR \va_i - \vt + \vv_{i, j}}^2}{\sigma^2}) \\
&\leq \exp(2\frac{(\norm{\vb_i - \MR \va_i - \vt} + \norm{ \vv_{i, j}})^2}{\sigma^2}) \\
&\leq \exp(2\frac{(\sqrt{3} \sigma + c \sigma)^2}{\sigma^2}) \\
&= \exp(2(\sqrt{3} + c)^2),
\end{align}
if we make sure that 
$$
\frac{\pi_1}{\pi_j} \geq \alpha \geq 8 \exp(2(\sqrt{3} + c)^2),
$$
we will have the likelihood of cluster 1 always greater than any other cluster so that all the points will cluster into 1. We need 
$$
c \leq \sqrt{\frac{1}{2} \log{\frac{\alpha}{8}}} - \sqrt{3}.
$$

Recall that \Cref{lem:HornRepeat} states that 
\begin{align*}
\|\hat \MR - \MR\|_F^2 \leq \frac {18 B \sigma}{\lambda_{min}(\MSigma)}\sqrt{\frac{2}{m} \log \frac {18} \delta }
\end{align*}
and,
\begin{align*}
\| \hat \vt - \vt \|_2^2 \leq  36 B \sigma  \sqrt{\frac{2}{m} \log \frac {\textcolor{black}{18}} \delta } +
\frac{12}{m} \sigma^2 \log \frac {\textcolor{black}{6}} \delta 
\end{align*}
Since the largest final error of $\vv_{i,j} = \norm{\vb_i - \MR_j \va_i - \vt_j}^2$ for all $i$ is bounded by the largest possible error given by \Cref{lem:HornRepeat}, then $\max_i \|\vv_{i,j}\|$ may be bounded by $\frac {18 B^2 \sigma}{\lambda_{min}(\MSigma)}\sqrt{\frac{2}{m} \log \frac {\textcolor{black}{18}} \delta } + 36 B \sigma  \sqrt{\frac{2}{m} \log \frac {\textcolor{black}{18}} \delta } +
\frac{12}{m} \sigma^2 \log \frac {\textcolor{black}{6}} \delta$. 
Then, we have $c \leq \frac {18 B^2 }{\lambda_{min}(\MSigma)}\sqrt{\frac{2}{m} \log \frac {\textcolor{black}{18}} \delta } + 36 B  \sqrt{\frac{2}{m} \log \frac {\textcolor{black}{18}} \delta } + \frac{12}{m} \sigma \log \frac {\textcolor{black}{6}} \delta$. To let $c \leq \sqrt{\frac{1}{2} \log{\frac{\alpha}{8}}} - \sqrt{3}$, we need 
$$
\frac {18 B^2 }{\lambda_{min}(\MSigma)}\sqrt{\frac{2}{m} \log \frac {\textcolor{black}{18}} \delta } + 36 B  \sqrt{\frac{2}{m} \log \frac {\textcolor{black}{18}} \delta } + \frac{12}{m} \sigma \log \frac {\textcolor{black}{6}} \delta \leq \sqrt{\frac{1}{2} \log{\frac{\alpha}{8}}} - \sqrt{3}
$$
We will solve for $m$ satisfying (1) $\frac {18 B^2}{\lambda_{min}(\MSigma)}\sqrt{\frac{2}{m} \log \frac {\textcolor{black}{18}} \delta }  < \frac 1 3 (\sqrt{\frac{1}{2} \log{\frac{\alpha}{8}}} - \sqrt{3})$, (2) $36 B  \sqrt{\frac{2}{m} \log \frac {\textcolor{black}{18}} \delta } < \frac 1 3 (\sqrt{\frac{1}{2} \log{\frac{\alpha}{8}}} - \sqrt{3})$ and (3) $\frac{12}{m} \sigma \log \frac {\textcolor{black}{6}} \delta < \frac 1 3 (\sqrt{\frac{1}{2} \log{\frac{\alpha}{8}}} - \sqrt{3})$. Any $m$ simultaneously satisfying (1), (2), and (3) will give us our result. To this end, we just choose $m_0$ to be the largest of these $m$.
By enforcing
$m_0 \geq 2.5 \cdot 10^4 \log \frac{18}{\delta} \max 
\{ \frac{B^4}{\lambda^2},  B^2 , \sigma\} (\frac 1 2 \log \frac{\alpha}{8})^{-\frac 1 2}
% > 
% 2.5 \cdot 10^8 \max \{\frac{B^4}{\lambda^2} (\frac{\alpha+1}{\alpha-1})^2 \log \frac {18} {\delta},  B^2 
% (\frac{\alpha+1}{\alpha-1})^2 \log \frac{18}{\delta}, \sigma \frac{\alpha+1}{\alpha-1}
% \log \frac{6}{\delta}, \\ 0.1 \log \frac{2}{\delta} \}
$, 
we have upper bounded $c$ with probability $1-\delta$ such that 
$$
c \leq \sqrt{\frac{1}{2} \log{\frac{\alpha}{8}}} - \sqrt{3},
$$
which implies the cluster with $j=1$ will always have the largest likelihood for all points. This means $\pi_1$ keeps increasing in size in each iteration and eventually all the elements of $G_1$ will collect into $H_1$.
\qed
