# Supplementary material for: Learning Correspondence for Deformable Objects
Source: arXiv:2405.08996 source file (2024-05-28)
Supplement: Supplementary file 4 [file appendix2_backup.tex]

\begin{theorem}[Expectation-Maximization Guarantee]
\label{thm:EMrepeat}
In the setting of Definition \ref{set:problem}, 
assume that the initial clustering $\cH$ is 
$(\tau,\alpha,m_0)$-good in the sense of Definition \ref{def:initial_conditions}, where $m_0 \geq 2.5 \cdot 10^8  (\frac{\alpha+1}{\alpha-1})^2 \log \frac {18} {\delta} \max\left\{\frac{B^4}{\lambda^2},  B^2 , \sigma  \right\}$ 
% is some sufficiently large polynomial function of $1/\alpha, 1/\sigma_j$ and $\log(1/\delta)$, 
where $\delta$ is the probability of failure of the algorithm and $\lambda$ is the smallest eigenvalue of {$\frac 1 m \sum_i \va'_i (\va'_i)\tran$.}
Then, the partition $\cH'$ returned by \Cref{alg:EM} {recovers each of the ground truth clusters} (\eg the objects and background) with probability $1-\delta$.
% Then, running \Cref{alg:EM}, with probability $1-\delta$,
% returns $\cH'$, a partition of the set of correspondences $S$, {recovering each of the ground truth clusters} (\ie the objects and background). 
\end{theorem}
% We now sketch a proof outline of our main theoretical guarantee. 
% \emph{Intuition:}
% The proof of~\cref{thm:EM} follows by noting that the initial clustering results in a partition of each ground truth cluster such that one of the partitions is notably larger than the rest. 
% As the algorithm progresses, the M-step assigns more points to the biggest estimated cluster until it is exactly matches to the ground truth object which contains it. 
% This happens because the likelihood term $W_{i,j;\tau}$ is dominated by the weight term $\pi_j$ of the largest cluster. 

\emph{Proof:}
We make the following observations, which together imply that the final clusters produced by~\Cref{thm:EM}  recover the ground truth clusters. 
First, {each ground truth-cluster is partitioned by the initial clustering}. This is because
% one element of which is $\alpha$-times larger than all the others.
the $\tau$-connected subsets of the data either consist of samples that are entirely contained in one of the $G_j$ or (possibly) the set of outliers. Since the initial clustering $\cH$ exclusively consists of $\tau$-connected subsets, % and is a partition of $S$, 
each element of $\cH$ is either a subset of $G_j$ for some $j$ or entirely consists of outliers.

Now %now set up some convention for what follows.
suppose the weights for the clusters are given by $\pi_1, \dots, \pi_{K}$.
Without loss of generality, suppose $\{ H_1, \dots, H_t \}$ form a partition of $G_1$ 
with $\pi_1 \geq \dots \geq \pi_{t}$. Since $\cH$ is $(\tau,\alpha, m_0)$-good,
we know that $\pi_1 > \alpha \pi_2$ because of \Cref{item:identifying-cluster} in Definition~\ref{def:initial_conditions}. 
Our second claim is that in each iteration of the $M$-step,
elements of $S$ that are $\tau$-close to the largest cluster $H_1$ are assigned to $H_1$. 
To see this, consider a point $(\va_i, \vb_i) \in G_1 \setminus H_1$ which is $\tau$-close to $H_{1}$ (if no such point exists, then $H_1 = G_1$). We show that for the point $(\va_i, \vb_i)$, the likelihood term $W_{i,j;\tau}$ is maximized when $j=1$. 
% This will follow from the fact that $W_{i,1;\tau}$ is much larger than $W_{i,j;\tau}$ for all $j\in[t] \setminus \{1\}$ because $\pi_1$ is much larger than the weights for the other clusters.


% Since Horn's Method is consistent (to be consistent means that with a sufficiently large sample size, the algorithm converges to the true solution in the presence of zero-mean  noise) and the domain of the point-cloud is bounded by a ball of radius $B$, 
% $(\hat{\MR}_j^{(r)}, \hat{\vt}_j^{(r)})$ and $\sigma'_j$ estimates $(\MR_j^{(r)}, \vt_j^{(r)})$ and $\sigma_j$ up to an additive error of $\eta_j'$. Let $m_0 := \frac
% {2 \log \frac 2 \delta}
% {(-\frac{4B}{\sigma_j} -\frac{2 B^2}{\sigma_j \lambda} +  \sqrt{(\frac{4B}{\sigma_j} + \frac{2 B^2}{\sigma_j \lambda} )^2 - \frac{1}{2400} \frac{1-\alpha}{1+\alpha} \frac{1}{\sigma_j} })^2}$.

% \red{A large sample size can be ensured by letting $m_0$ be a sufficiently large polynomial function of $1/\eta', 1/\sigma_j$, and $\log(1/\delta)$, where $\delta$ is the probability of success.} 
% Then, for all $H_j$ such that $|H_j|$ is large enough, our estimates $h_j$ and $\sigma'_j$ converge to the corresponding ground truth parameters ($g_1$ and $\sigma_j$).

% However, if $|H_j|$ is much smaller than $m_\min$ \new{as defined in our algorithm}, we delete the cluster $H_j$ from our set of candidate clusters. 

Notice that 
$\argmax_j W_{i,j;\tau} 
= \argmax_j \pi_j \phi_j(\vb_i \mid \va_i) 
= \argmax_j \pi_j \exp(-\norm{\vb_i - \hat{\MR}_j\va_i - \hat{\vt}_j }^2/{\hat\sigma_j}^2) /\hat\sigma_j$ (where we dropped constants that are inconsequential for the maximization). 
\LC{missing $\frac{1}{2}$ (does it matter?) and $\hat\sigma_j$ should be $\hat\sigma_j^3$}

Let $\vv_{i, j} := \hat{\MR}_j \va_i + \hat{\vt}_j - (\MR_j \va_i + \vt_j)$, 
let $\sigma_j$ be the variance for the noise, \ie \red{fill in},
and $\eta_j' := \max{\{\max_i \|\vv_{i, j}\|,  |\sigma_j - \hat\sigma_j|\}}$.
Let $c := \eta_j' / \sigma_j$, so that $C = 1/(1 \pm c)=1 \pm (c/2)$.
Then, we have
\begin{align}
&\quad \frac{\pi_j}{\sigma'_j} \exp\left(-\frac{\norm{\vb_i - \hat{\MR}_j \va_i - \hat{\vt}_j }^2}{ (\sigma'_j)^2}\right) \\
&= \frac{\pi_j}{\sigma_j \pm \eta_j'} \exp(-\frac{\norm{\vb_i - \MR_j \va_i - \vt_j + \vv_{i, j}}^2}{(\sigma_j \pm \eta_j')^2}) \\
&= \frac{C\pi_j}{\sigma_j} \exp(-\frac{C^2\norm{\vb_i - \MR_j \va_i - \vt_j + \vv_{i, j}}^2}{\sigma_j^2}) \\
&= \frac{C\pi_j}{\sigma_j} \exp(-C^2\frac{2 \vv_{i, j} \cdot (\vb_i - \MR_j \va_i - \vt_j) + \norm{\vv_{i, j}}^2}{\sigma_j^2})  \\
&\quad \cdot \exp(-C^2\frac{\norm{\vb_i - \MR_j \va_i - \vt_j}^2}{\sigma_j^2}) \\
&= \frac{C\pi_j}{\sigma_j} \exp(-C^2\frac{2 \vv_{i, j} \cdot (\vb_i - \MR_j \va_i - \vt_j) + \norm{\vv_{i, j}}^2}{\sigma_j^2})  \\
&\quad \cdot  \exp(-(2(C-1) + (C-1)^2)\frac{\norm{\vb_i - \MR_j \va_i - \vt_j}^2}{\sigma_j^2}) \\
&\quad \cdot \exp(-\frac{\norm{\vb_i - \MR_j \va_i - \vt_j}^2}{\sigma_j^2})
% &= \frac{\pi_j}{\sigma'_j \pm \eta'} \exp(-\norm{\vb_i - R_j \va_i - \vt_j \pm \eta') }^2/(\sigma'_j \pm \eta')^2) \\
% &= C \frac{\pi_j}{\sigma'_j} \exp(-C^2 \norm{\vb_i - R_j \va_i - \vt_j \pm \eta') }^2/\sigma'_j^2\\
% &= C \frac{\pi_j}{\sigma'_j} \exp(-C^2 \norm{\vb_i - R_j \va_i - \vt_j \pm \eta') }^2/\sigma'_j^2\\
\end{align}

Lemma~\ref{lem:close_to_1} shows that except for $(\pi_j/\sigma_j)~\exp(-\frac{\norm{\vb_i - \MR_j \va_i - \vt_j}^2}{\sigma_j^2})$, all the other terms take values in $[1 - 33 c, 1 + 33 c]$. 
\begin{lemma}\label{lem:close_to_1}
In the setting of \Cref{thm:EM}, if $C = 1 \pm (c/2)$, $c = \eta_j'/\sigma_j \in (0, 0.03)$, then \\
$C \cdot \exp(-C^2~\frac{( 2 \vv_{i, j}) \cdot (\vb_i - \MR_j \va_i - \vt_j) + \norm{\vv_{i, j}}^2}{\sigma_j^2}) \cdot \exp(-(2(C-1) + (C-1)^2)~\frac{\norm{\vb_i - \MR_j \va_i - \vt_j}^2}{\sigma_j^2}) \in [1 - 33 c, 1 + 33 c]$. 
\end{lemma}
\begin{proof}
We already know that $C = 1\pm (c/2)$. We will show the following:\\
(1) $|1 - \exp(-C^2~\frac{(2 \vv_{i, j}) \cdot (\vb_i - \MR_j \va_i - \vt_j) + \norm{\vv_{i, j}}^2}{\sigma_j^2})| \leq 21 c$, \\
(2) $|1 - \exp(-(2(C-1) + (C-1)^2)~\frac{\norm{\vb_i - \MR_j \va_i - \vt_j}^2}{\sigma_j^2})| \leq 9 c$. \\
To this end, we will need the following fact: for all $|p| \leq 1$,   $1 - 2|p|\leq \exp(p) \leq 1+ 2 |p|$. \\
Also note that since the noise is bounded in absolute value by $\sigma_j$, we have $\norm{\vb_i - \MR_j \va_i - \vt_j} < \sqrt{3} \sigma_j$. 
% We will show that $\exp(-C^2~\frac{(\pm 2 \eta') \cdot (\vb_i - R_j \va_i - \vt_j) + \norm{\eta'}^2}{\sigma_j^2}) = 1 +\eta_1$ and $\exp(-(2(C-1) + (C-1)^2)~\frac{\norm{\vb_i - R_j \va_i - \vt_j}^2}{\sigma_j^2}) = 1+\eta_2$ such that $\eta_1, \eta_2$ are both $O(c)$ where 
Together, these imply, 
\begin{align}
&\left|1-\exp\left(-C^2~\frac{(2 \vv_{i, j}) \cdot (\vb_i - \MR_j \va_i - \vt_j) + \norm{\vv_{i, j}}^2}{\sigma_j^2}\right)\right|\\
&\leq 2\left |-C^2~\frac{(2 \vv_{i, j}) \cdot (\vb_i - \MR_j \va_i - \vt_j) + \norm{\vv_{i, j}}^2}{\sigma_j^2} \right| \\
& \leq 2C^2 \left ( \left |\frac{2 \vv_{i, j} \cdot (\vb_i - \MR_j \va_i - \vt_j)}{\sigma_j^2}\right| + \frac{\norm{\vv_{i, j}}^2}{\sigma_j^2}\right) \\
& \leq 2C^2 \left (\frac{2 \norm{\vv_{i, j}} \norm{\vb_i - \MR_j \va_i - \vt_j}}{\sigma_j^2} + \frac{\norm{\vv_{i, j}}^2}{\sigma_j^2}\right) \\
& \leq 2C^2 \left (\frac{2 \eta'_j \norm{\vb_i - \MR_j \va_i - \vt_j}}{\sigma_j^2} + \frac{(\eta'_j)^2}{\sigma_j^2}\right) \\
% & \leq 2C^2 \left (\frac{2 \norm{\eta'} \sqrt{3} \sigma_j}{\sigma_j^2} + \frac{\norm{\eta'}^2}{\sigma_j^2} \right) \\
% & \leq 2C^2 \left (\frac{2 \sqrt{3} \norm{\eta'}}{\sigma_j} + \frac{\norm{\eta'}^2}{\sigma_j^2} \right)\\
& \leq 2C^2 \left (2 \sqrt{3} c + c^2 \right) \\
& \leq 21 c
% \frac{2 \sqrt{3} \norm{\eta'}}{\sigma_j} + \frac{\norm{\eta'}^2}{\sigma_j^2} \right)
\end{align}
Similarly, we can show that
\begin{align}
&\left | 1-\exp\left(-(2(C-1) + (C-1)^2)~\frac{\norm{\vb_i - \MR_j \va_i - \vt_j}^2}{\sigma_j^2}\right) \right|\\
% &\leq 2\left|-(2(C-1) + (C-1)^2)~\frac{\norm{\vb_i - R_j \va_i - \vt_j}^2}{\sigma_j^2}\right| \\
&\leq |(4(C-1) + 2(C-1)^2)~\frac{3 \sigma_j^2}{\sigma_j^2}| \\
&\leq |6 c + 3c^2| \\
&\leq 9 c
\end{align}
Putting everything together,
% $\frac{c}{c \pm 1} = 1 - \frac{\eta'/\sigma_j}{\eta'/\sigma_j \pm 1} = 1 - \frac{\eta'}{\eta' \pm \sigma_j} = 1 + \eta_0$. 
we have $C \cdot \exp(-C^2~\frac{( 2 \vv_{i, j}) \cdot (\vb_i - \MR_j \va_i - \vt_j) + \norm{\vv_{i, j}}^2}{\sigma_j^2}) \cdot \exp(-(2(C-1) + (C-1)^2)~\frac{\norm{\vb_i - \MR_j \va_i - \vt_j}^2}{\sigma_j^2}) \in [(1 - (c/2)) (1 - 21c) (1 - 9c), (1 + (c/2)) (1 + 21c) (1 + 9c)] \in [1 - 33c, 1 + 33 c]$ for $c\in(0, 0.03)$.
\end{proof}
We choose $\eta_j'$ to be sufficiently small so that $33c  = 33 \frac{\eta'_j}{\sigma_j}\leq \frac{\alpha-1}{\alpha+1} $.
% To enforce this, i.e. that the final error is smaller than $\eta'_j \leq \frac{\sigma_j}{33} \frac{\alpha -1}{\alpha+1}$ we will bound each of the contributions to the final error according to  
Recall that \Cref{lem:HornRepeat} states that 
\begin{align*}
\|\hat \MR - \MR\|_F^2 \leq \frac {18 B \sigma_j}{\lambda_{min}(\MSigma)}\sqrt{\frac{2}{m} \log \frac {\textcolor{red}{18}} \delta }
\end{align*}
and,
\begin{align*}
\| \hat \vt - \vt \|_2^2 \leq  36 B \sigma_j  \sqrt{\frac{2}{m} \log \frac {\textcolor{red}{18}} \delta } +
\frac{12}{m} \sigma_j^2 \log \frac {\textcolor{red}{6}} \delta 
\end{align*}
Since the largest final error of $\vv_i = \norm{\vb_i - \MR_j \va_i - \vt_j}^2$ for all $i$ is bounded by the largest possible error given by \Cref{lem:HornRepeat} and $\sigma_j'$ is the standard deviation of the error, then $\eta_j' := \max{\{\max_i \|\vv_{i, j}\|,  |\sigma_j - \sigma'_j|\}} = \max_i \|\vv_{i, j}\|$. Then, this implies that the final error $\eta_j'$ may be bounded by $\frac {18 B^2 \sigma_j}{\lambda_{min}(\MSigma)}\sqrt{\frac{2}{m} \log \frac {\textcolor{red}{18}} \delta } + 36 B \sigma_J  \sqrt{\frac{2}{m} \log \frac {\textcolor{red}{18}} \delta } +
\frac{12}{m} \sigma_j^2 \log \frac {\textcolor{red}{6}} \delta$. We will solve for $m$ satisfying (1) $\frac {18 B^2 \sigma_j}{\lambda_{min}(\MSigma)}\sqrt{\frac{2}{m} \log \frac {\textcolor{red}{18}} \delta }  < \eta'/3$, (2) $36 B \sigma_j  \sqrt{\frac{2}{m} \log \frac {\textcolor{red}{18}} \delta } < \eta'/3$ and (3) $\frac{12}{m} \sigma_j^2 \log \frac {\textcolor{red}{6}} \delta < \eta'/3$. Any $m$ simultaneously satisfying (1), (2) and (3) will give us our result. To this end, we just choose $m_0$ to be the largest of these $m$.
which is enforced by 
$m_0 \geq 2.5 \cdot 10^8  (\frac{\alpha+1}{\alpha-1})^2 \log \frac{18}{\delta} \max 
\{ \frac{B^4}{\lambda^2},  B^2 , \sigma_j  \} > 
2.5 \cdot 10^8 \max \{\frac{B^4}{\lambda^2} (\frac{\alpha+1}{\alpha-1})^2 \log \frac {18} {\delta},  B^2 
(\frac{\alpha+1}{\alpha-1})^2 \log \frac{18}{\delta}, \sigma_j \frac{\alpha+1}{\alpha-1}
\log \frac{6}{\delta} \}$, 
using Theorem \ref{lem:HornRepeat}, we get, $|\eta_j| \leq 400c \leq \frac{\alpha -1}{\alpha+1}$.
% (\frac
% {24 \sigma_j \log \frac {18} {\delta}}
% {- ( \frac{18 B^2}{\lambda} + 36B) \sqrt{2 \log \frac{2}{\delta}} + \sqrt{( \frac{18 B^2}{\lambda} + 36B)^2 {2 \log \frac{2}{\delta}} + \frac {3} {25} \sigma_j (\log \frac{18}{\delta}) \frac{\alpha-1}{\alpha+1}}} )^2




% \new{Constraints: 
% 1. $\eta' = c \sigma_j$ then $C = 1/(1 \pm c)$.
% 2. $c$ can be chosen to be a sufficiently small constant (like $0.1$) since $\sigma_j =1$. This will reduce $\eta'$.
% The cost of this is the sample size. 


% }















 % we see that for a sufficiently large $H_j$ for $j \in [t]$, 
 % $h_j$ converges to $g_1$ on the domain of the point-cloud, 
 % i.e. $|h_j(\va_i) - g_1(\va_i)| \leq \eta'$. 

% Similarly, it can be shown that our estimate of the standard deviation of the noise is also correct upto an additive error of $\eta'$.
% true for our estimate of the standard deviation of the noise.

% Let $\sigma_j$ denote the standard deviation of the noise in $G_1$ with respect to the ground truth rotation and translation $g_1$. 
 
% (the bound on the norm of the elements of the point cloud). 

Since $\exp(-\norm{\vb_i - g_1(\va_i)}^2/{\sigma_j}^2)/\sigma_j$ is a constant with respect to $j$ in $\argmax_j W_{i,j;\tau}= \argmax_j \pi_j (1\pm \eta_j) \exp(-\norm{\vb_i - g_1(\va_i)}^2/{\sigma_j}^2)/\sigma_j$, it does not affect the maximization. 
This implies 
% $\argmax_j W_{i,j;\tau}=\argmax_j \pi_j (1\pm 3\eta)$, and so 
$\argmax_j W_{i,j;\tau}$ is essentially determined by $\argmax_j \pi_j (1\pm \eta_j)$. By letting large enough $m_0$ ,we have small $\eta_j$ to ensure $(1+\eta_j)/(1-\eta_j) < \alpha$ and recalling that $\pi_1 > \alpha \pi_2$, we see $\argmax_j W_{i,j;\tau} = \argmax_j \pi_j (1\pm \eta_j) = 1$. Since $\pi_1$ keeps increasing in size in each iteration, eventually all the elements of $G_1$ will collect into $H_1$. 

% $\exp(-\norm{g_1(\va_i) - \vb_i}^2/{{\sigma_j^*}_1}^2)/{\sigma_j^*}_1$ for $\eta$ chosen to be sufficiently small. Since the second term is a constant with respect to $j$, by choosing $\eta$ to be sufficiently small we can ensure $(1+\eta)/(1-\eta) < \alpha$, and so $\argmax_j W_{i,j;\tau} = \argmax_j \pi_j (1\pm \eta) = 1$. 
% (i.e. smaller than $(1-\alpha)(1/3)$)
% $\argmax_j W_{i,j;\tau} 
% = \argmax_j \pi_j \phi_j(\vb_i \mid \va_i) 
% = \argmax_j \pi_j \exp(-\norm{h_j(\va_i) - \vb_i}^2/{\sigma'_j}^2)/\sigma'_j 
% = \argmax_j \pi_j (1\pm \eta') \exp(-\norm{g_1(\va_i) - \vb_i}^2/{{\sigma_j^*}_1}^2)/{\sigma_j^*}_1 
% = 1$. 
% The second-to-last equality is a consequence of choosing $\eta$ sufficiently small,
% and $\eta'$ satisfying $1+\eta' < \alpha$. 
\qed
% To see this, observe that since each $H_i$ is sufficiently large, 
% with high probability,
% Horn's method will converge to the true rotation $g_1$,
% and our estimate of the standard deviation of the noise in each of the partitions will be close to the standard deviation of the noise with respect to $g_1$ for the samples in $G_1$.
% A short calculation then demonstrates that $\argmax_j W_{i,j;\tau}$ is essentially determined by $\argmax_j \pi_j (1\pm 3\eta)$ when $\eta$ is small enough. Choosing $\eta$ to ensure $(1+\eta)/(1-\eta) < \alpha$ and recalling that $\pi_1 > \alpha \pi_2$, we see $\argmax_j W_{i,j;\tau} = \argmax_j \pi_j (1\pm \eta) = 1$. Since $\pi_1$ keeps increasing in size in each iteration, eventually all the elements of $G_1$ will collect into $H_1$. 

% Since each $H_i$ is sufficiently large, with high probability,
% Horn's method will converge to the true rotation $g_1$,
% and our estimate of the standard deviation of the noise in each of the partitions will be close to the standard deviation of the noise with respect to $g_1$ for the samples in $G_1$.

% \red{
% satisfying certain conditions (which we observe in our experiments),
% namely, (i) $\cH$ is a partition of $S$;
% (ii) Every ground truth cluster contains at least one cluster from $\cH$ that is relatively large compared to the others; and
% (iii) Every cluster in the initial clustering is not too small, and is $\tau$-connected.
% \myparagraph{Preliminaries and Notation}
% We provide the following notation and definitions that we will use in this and the following section. 

% \blue{Sushrut: Removed even more calculation, hopefully this is okay.}



% The final equality follows from the facts that (i) the partitions are independent of the noise
% (ii) both Horn's method and the empircal estimate of the standard deviation are consistent, 
% and converge to the true mean.

% It is easy to see that if $\pi^{(r)}_q < (1-3\eta)\pi^{(r)}_{i^*}$, 
% then then all the samples in $H_q$ will be reassigned to $H_{i^*}$.

% \emph{Noiseless setting:}



% \emph{With Noise:}

% Our proof proceeds in $2$ steps:

% First, the initial clustering $\cH := \{ H_1, \dots, H_{M} \}$ is such that each of the $H_i$ is either a subset of $G_j$ for some $j$ or entirely consists of outliers.
% This is because the only $\tau$-connected subsets of the data either consist of samples that are entirely contained in one of the $G_i$ or (possibly) the set of outliers. 
% Second, In each iteration, the mass on the ground truth clusters concentrates. 

% To see this, suppose that during the $r^{th}$ iteration,
% the weights for the $M$ hypotheses are given by $\pi^{(r)}_1, \dots, \pi^{(r)}_{M}$.
% Let $i^* := \argmax_i \pi_i^{(r)}$. 
% Of these, suppose without loss of generality that for some $t \geq 1$, 
% hypotheses $H_1, \dots, H_t \subset G_1$,
% and $\cup_{i=1}\tran H_i = G_1$. 
% Then, 
% \begin{enumerate}
%     \item If $\pi^{(r)}_{i^*}$ is sufficiently large (larger than $(1+3\eta)$ times the second largest in the set $\{ \pi_i^{(r)} \}_{i=1}^{M}$), then in the M-step, every sample that is $\tau$-close to  $H_{i^*}$ gets assigned to $i^*$. \label{item:large_sufficient}
%     \item Since each of the ground-truth sets are $\tau$-connected, there are always samples close to the largest cluster which will keep getting accumulated. 
%     \item Since the noise $\eta$ is much smaller than $\tau$, we see that the variance cannot 
% \end{enumerate}
%     To see \Cref{item:large_sufficient}, observe that 
%     This is because for any $(\va_i, \vb_i)$ which is $\tau$-close to $H_{i^*}$, 
%     $\argmax_j W^{(r)}_{i,j;\tau} 
%     = \argmax_j \pi^{(r)}_j \phi^{(r)}_j(\vb_i \mid \va_i) 
%     = \argmax_j \pi^{(r)}_j \exp(\norm{h_j(\va_i) - \vb_i}^2/{\sigma_j^{(r)}_j}^2)/\sigma_j^{(r)}_j = \argmax_j \pi^{(r)}_j (1\pm \eta) \exp(\norm{g_1(\va_i) - \vb_i}^2/{{\sigma_j^*}_1}^2)/{\sigma_j^*}_1 
%     = i^*$. 
%     The final equality follows from the fact that 
%     each of the $h_j$ are 


% Then, it is easy to see that if some point $(\va_i, \vb_i) \in H_1$, 
% line $18$ of the algorithm will assign the point $p_j$ to the hypothesis indexed by $f(i) := \argmax_j W_{i,j;\tau}^{(r)}$. 
% The convention the algorithm uses is that $f(i)$ will be the smallest index
% among all the possible candidates which achieve the largest value. 
% We will show that if $\pi^{(r)}_1$ is sufficiently large,
% then all the mass gets concentrated in $H_1$.
% If this is not the case, then $\pi^{(r)}_1$ will eventually
% become sufficiently large. 
% To see the first claim, we make the following observations: 
% (i) Since each $H_i$ is sufficiently large, and independent of the noise. The sample variance of each of the sets $H_1, \dots, H_t$, $\sigma_j^{(r)}_{i} = \sigma_j_1 (1 \pm \etailon)$. 
% (ii) If $\pi^{(r)}_1 \geq (1+\eta) \pi^{(r)}_{2}$, then every sample in $H_1 \cup \dots \cup H_t$ goes to $H_1$. 


% $
% = \argmax_j  \frac{ \pi_j^{(r)}\phi_k^{(r)}(\vb_i | \va_i)}{\sum_{j=1}^g \pi_j^{(r)} \phi_j^{(r)}(\vb_i | \va_i) } 
% \cdot \mathbf{1}(d_{\text{cluster}}(H_j, (\va_i, \vb_i)) < \tau)$.
% This is nonzero only if the distance from $H_j$ to  $(\va_i, \vb_i)$ is at most $\tau$.
% This ensures that the point $(\va_i, \vb_i)\in G_1$ 
% cannot be assigned to any $G_j$ where $j \neq 1$. 
% If the value is indeed nonzero, then in the next iteration $r+1$, 
% the point $(\va_i, \vb_i)$ will be assigned to the hypothesis $H_j$
% where $j = \argmax_{j \in [t]} \pi_j^{(r)}\phi(0,{\sigma_j^{(r)}}_j^2)$.
% We put the hypothesis in the smallest index cluster if all entries are the same.
% However, since with probability 
% \snote{1. show big clusters get bigger. 
% 2. If equal sized cluster then the preference is to a lower index.}

% Since $|H_i| \geq \Omega(\frac{1}{\eta^2} \log(1/\delta))$ we know that Horn's Method recovers a hypothesis $h_i$ that is close to $g_j$ (see \cite{}). 
% \snote{don't talk about $h_i$, these will keep getting updated later. $H_i$ depends on the original noise gaussian}

% \hide{\new{
% We will show that given a good initialization,
% it is possible to recover the right hypotheses.
% To this end, we demonstrate the following.

% \emph{1. The ``good hypotheses" are never eliminated:}
% To see this, observe that the error a point $\vp$ makes with respect to the target hypothesis is small.
% This is because the rotations are well-separated. 
% Additionally, note that the likelihood of such a point is going to be nonzero.


% \emph{2. Any hypothesis that makes an error of more than $10\tau$ with the original hypothesis is eliminated.}
% To see this, suppose to the contrary that there is an h which is far from all the $g_1, .., g_|G|$.but makes an error of $\leq \tau$ for each of these.This means there is at least one $G_i$ which overlaps with $h$ significantly.
% But this means $h(x) - y = g(x) - y \pm \tau$ and so $h(x) - g(x) = O(\tau)$.
% but this in turn means that $h$ and $g$ are close.so the number of points that $h$ explains has to be smaller than \new{???}.If so, it gets eliminated..

% \emph{3. Among the good hypotheses the points that correspond to that object eventually collect}
% Let the ground truth be let $p \in G_i$ and suppose the samples are


% \snote{Need to first find weights, then cluster together etc. This will help collect things. Which will eventually converge. }

% }
% We will discuss this in the noiseless setting first.

% \paragraph{Noiseless}

% We know from the setting of the problem (\Cref{set:problem})
% that $|G_i| \geq \gamma |S|$. 

% Let $\cH_{\geq}$ denote the subset of $\cH$ such that for every $h \in \cH_{\geq}$,
% $|H_0(h)| \geq \gamma |S|$, where 
% $H_\eta(h) := \{ (x, y) \in S \mid \err(h; \{(x, y)\}) \leq \eta \}$. 
% Now, since $S$ is partitioned into $G_1, \dots, G_k$, 
% it must be the case that each $H_0(h)$ has some overlap with some of the $G_i$. 
% Since the setting is non-degenerate (\Cref{item:NdO} from \Cref{set:problem}), 
% If $|H_0(h) \cap G_i| \geq (d+1)$ where $d$ is the dimension (in our case a constant),
% then $h \equiv g_i$. 
% Otherwise $|H_0(h)| \leq (d+1) k$. 
% However, since $m > (d+1) k/\gamma$, and $|H_0(h)| \geq \gamma |S|$,
% we see that $h \notin \cH'$.
% Hence every $h \in \cH'$ is a ground truth hypothesis.
% Also, no ground truth hypothesis is removed, since $G_i \subset H_0(g_i)$ for every $i \in [k]$. \snote{$\cH'$ and $\cH_{\geq}$. Make them the same.}

% \paragraph{Randomly Selected Arbitrary Outliers}

% Suppose an $\eta$ fraction of the samples $S$ are corrupted arbitrarily,
% but the location of these corruptions is uniform at random
% (this ensures that no object gets completely hidden).

% In the absence of any other noise, the previous argument still goes through.
% \snote{Okay, but how will you ensure good initial estimates via clustering?
% I think the right clustering strategy will not cluster the outliers with the inliers
% unless they are close to being inliers, in which case it does not matter.}
% Let $I$ denote the set of inliers, and $O$ the set of outliers, and $I \cup O = S$.
% If a hypothesis $h$ satisfies 
% $|H_0(h) \cap H_0(g)| \geq \Omega((d+1)/(1-\eta) \log(1/\delta))$ for some $g \in \cG$, 
% then, with probability $1-\delta$, $|H_0(h) \cap H_0(g) \cap I| \geq \Omega(d+1)$. 
% in which case, $h \equiv g$. 
% If there is no $g$ for which $|H_0(h) \cap H_0(g)| \geq \Omega((d+1)/(1-\eta) \log(1/\delta))$,
% then it must be that $|H_0(h)| \leq O((k (d+1) / (1-\eta)) \log(1/\delta))$.
% As long as $|S|$ is large enough, once again, 
% we have a contradiction and $h$ should have been removed.
% \snote{also consider adversarial noise}

% \new{\paragraph{Bounded Additive Noise}

% Suppose each $g_i$ satisfies $\err(g_i; G_i) \leq \eta$. 
% We know from the setting of the problem (\Cref{set:problem}) 
% that $|G_i| \geq \gamma |S|$. 
% Let $\cH_{\geq}$ denote the subset of $\cH$ such that for every $h \in \cH_{\geq}$,
% $|H_\eta(h)| \geq \gamma |S|$.

% Now, since $S$ is partitioned into $G_1, \dots, G_k$, 
% it must be the case that each $H_\eta(h)$ has some overlap with some of the $G_i$. 

% Since the setting is non-degenerate (\Cref{item:NdO} from \Cref{set:problem}), 
% \new{If $|H_\eta(h) \cap G_i| \geq \gamma' |S|$ then $\err(h, G_i) \leq (\gamma/\gamma')$.} 
% Otherwise $|H_\eta(h)| \leq \gamma' k |S|$. 
% However, since $m > |S|/k\gamma'$, and $|H_\eta(h)| \geq \gamma |S|$,
% we see that $h \notin \cH'$.
% Hence every $h \in \cH'$ is a ground truth hypothesis.

% Also, no ground truth hypothesis is removed, 
% since $G_i \subset H_\eta(g_i)$ for every $i \in [k]$. 
% Suppose each for every $g \in \cG$ we have $|H_\eta(h) \cap H_\eta(g)| \leq \alpha |S|$
% and so $|H_\eta(h)| \leq k \alpha |S|$. }
% }

% \end{proof}
